# Supplementary material for: Deep combinatorial optimisation for optimal stopping time problems : application to swing options pricing
Source: arXiv:2001.11247 source file (2021-01-08)
Supplement: Supplementary file 1 [file appendix.tex]

\appendix
